# Supplementary material for: Bayesian modelling of visual discrimination learning in mice
Source: arXiv:2301.02659 source file (2022-11-15)
Supplement: Supplementary file 1 [file 99-APPENDIX.tex]

% \begin{appendices}
% \chapter{}
% \section{Speed figures} \label{sec:APPX: lick}
% \section{Lick location figures}\label{sec:APPX: speed}
% \end{appendices}
